# Supplementary material for: Behind Maya: Building a Multilingual Vision Language Model
Source: arXiv:2505.08910 source file (2025-05-15)
Supplement: Supplementary file 1 [file X_suppl.tex]

\clearpage
\setcounter{page}{1}
\maketitlesupplementary

\section{Additional Results}
\label{sec:additional_results}
We compare Maya's responses with those of LLaVA-7B and GPT4 using a set of additional images. The objective is to qualitatively evaluate Maya's performance against a model of similar scale (LLaVA-7B) and a significantly larger model (GPT4, which is estimated to have trillions of parameters).The comparison includes examples of visual question answering and detailed caption generation to illustrate the strengths and differences among the models.

\noindent{\textbf{Visual Question Answering.}} Figure~\ref{fig:model_responses023} presents a comparative analysis of model responses to a visual question identifying the brand featured in an advertisement. The conversation box displays the outputs from three models: Maya, LLaVA-7B, and GPT4. All three models successfully identify the brand as ``Subway". Maya demonstrates a consistent understanding of visual content and excels at extracting OCR information, particularly when the text is clearly visible and occupies a significant portion of the image.

Figure \ref{fig:model_responses001} presents a comparative analysis of model responses in identifying a well known landmark. While LLaVA-7B and GPT4 correctly identify the landmark as ``Diamond Head", a volcanic crater in Hawaii, Maya incorrectly identifies it as the ``Seven Islands of Hawaii". This discrepancy illustrates differences in the models' accuracy and contextual understanding. The correct responses from LLaVA-7B and GPT4 demonstrate superior alignment with the visual and textual context, whereas Maya's misidentification suggests potential limitations in training on geographically specific datasets.

\noindent{\textbf{Caption Generation.}}
Our example in Figure \ref{fig:model_responses024_01} illustrates how Maya generates a description to a highways-at-night scene. All models provide a detailed description of the photo with different focuses. GPT4 provides precise information about the photo, including the number of lanes, the direction of the traffic, the density of the cars, the elevation of the four-lane highway, the illumination of the lights, and the presence of trees. Maya (similar to LLaVA-7B), while does not identify the number of lines, provides a vivid but detailed description of the scene.  

Next, we focus on models' ability to describe a culturally diverse image in Figure \ref{fig:model_responses022}. Here, GPT4 accurately identify the restaurant that serves this ramen, with detailed in the photo such as chashu in the ramen, the chopsticks in their paper wrap, the garnish, and the sides served with the ramen. It shows an understanding of the context. While Maya correctly identifies different elements on the table, the description is unfortunately lacks the specific culturally relevant details provided in the context. 

\noindent{\textbf{Caption Generation in Multilingual.}}
In Figure \ref{fig:food_in_details}, we compare Maya's response in 10 languages in describing the image in Figure \ref{fig:model_responses022} in detail. Translating Hindi response to English: \textit{The image shows a dining table with three bowls containing different Asian dishes. One of the bowls has noodles, which looks like a delicious soup. The other two bowls contain different types of  vegetables, making the meal healthy and vibrant. Apart from the main dishes, there are three cups on the table, probably for beverages.  A spoon is also visible, placed near the bowl of noodles, suggesting it will be used for serving the food. Overall, this scene captures a delectable and welcoming Asian dining experience}. In Chinese, Maya describes the scene as featuring \textit{a few bowls of Asian noodles of varying kinds}, along with identifying meat, vegetables, and a spoon. It also notes the presence of \textit{three cups possibly containing side dishes or drinks}, adding that \textit{the whole scene creates an inviting atmosphere for people to enjoy this delicious meal together}. English translation of Spanish response: \textit{The image shows a dining table with three bowls filled with different types of food, probably of Asian origin. One of the bowls appears to be a bowl of noodles, while the others contain a variety of vegetables. There are also three cups placed around the table, which adds to the variety of the meal.  A spoon can be seen resting on the table, ready to be used to enjoy the meal. The table is filled with delicious dishes, making it a welcoming scene for those who want to enjoy a meal together}. Bengali response is similar to Spanish - they both fail to identify matcha, meat and does not identify the correct position of the spoon. 

\begin{figure*}[h]
   \centering
   \begin{conversationbox}{Subway}
       \includegraphics[width=1\linewidth]{sec/assets/023.jpg}
        
       \textbf{Question:} \\
       What brand is featured in this advertisement? 
       \tcblower
       \textbf{Maya:} \\
       The Subway brand is featured in this advertisement.\\
       \textbf{LLaVA-7B:} \\
       The brand featured in this advertisement is Subway.\\
       \textbf{GPT4:} \\
       The brand featured in this advertisement is Subway.
   \end{conversationbox}
   \caption{Comparison of model responses to visual questions on brand recognition.}
   \label{fig:model_responses023}
\end{figure*}

\begin{figure*}[h]
   \centering
    %Main Question 1 with image
   \begin{conversationbox}{Diamond Head in Hawaii}
       \includegraphics[width=1\linewidth]{sec/assets/001.jpg}
        
       \textbf{Question:} \\
       What is the name of this famous sight in the photo? 
       \tcblower
       \textbf{Maya:} \\
       The famous sight in the photo is the Seven Islands of Hawaii.\\
       \textbf{LLaVA-7B:} \\
       The famous sight in the photo is the Diamond Head, which is a volcanic crater located in Hawaii.\\
       \textbf{GPT4:} \\
       The famous sight in the photo is Diamond Head.
   \end{conversationbox}
   \caption{Comparison of model responses to visual questions on identifying famous landmark.}
   \label{fig:model_responses001}
\end{figure*}

\begin{figure*}[h]
    \centering
    \begin{conversationbox}{Highways at Night}
        \includegraphics[width=1\linewidth]{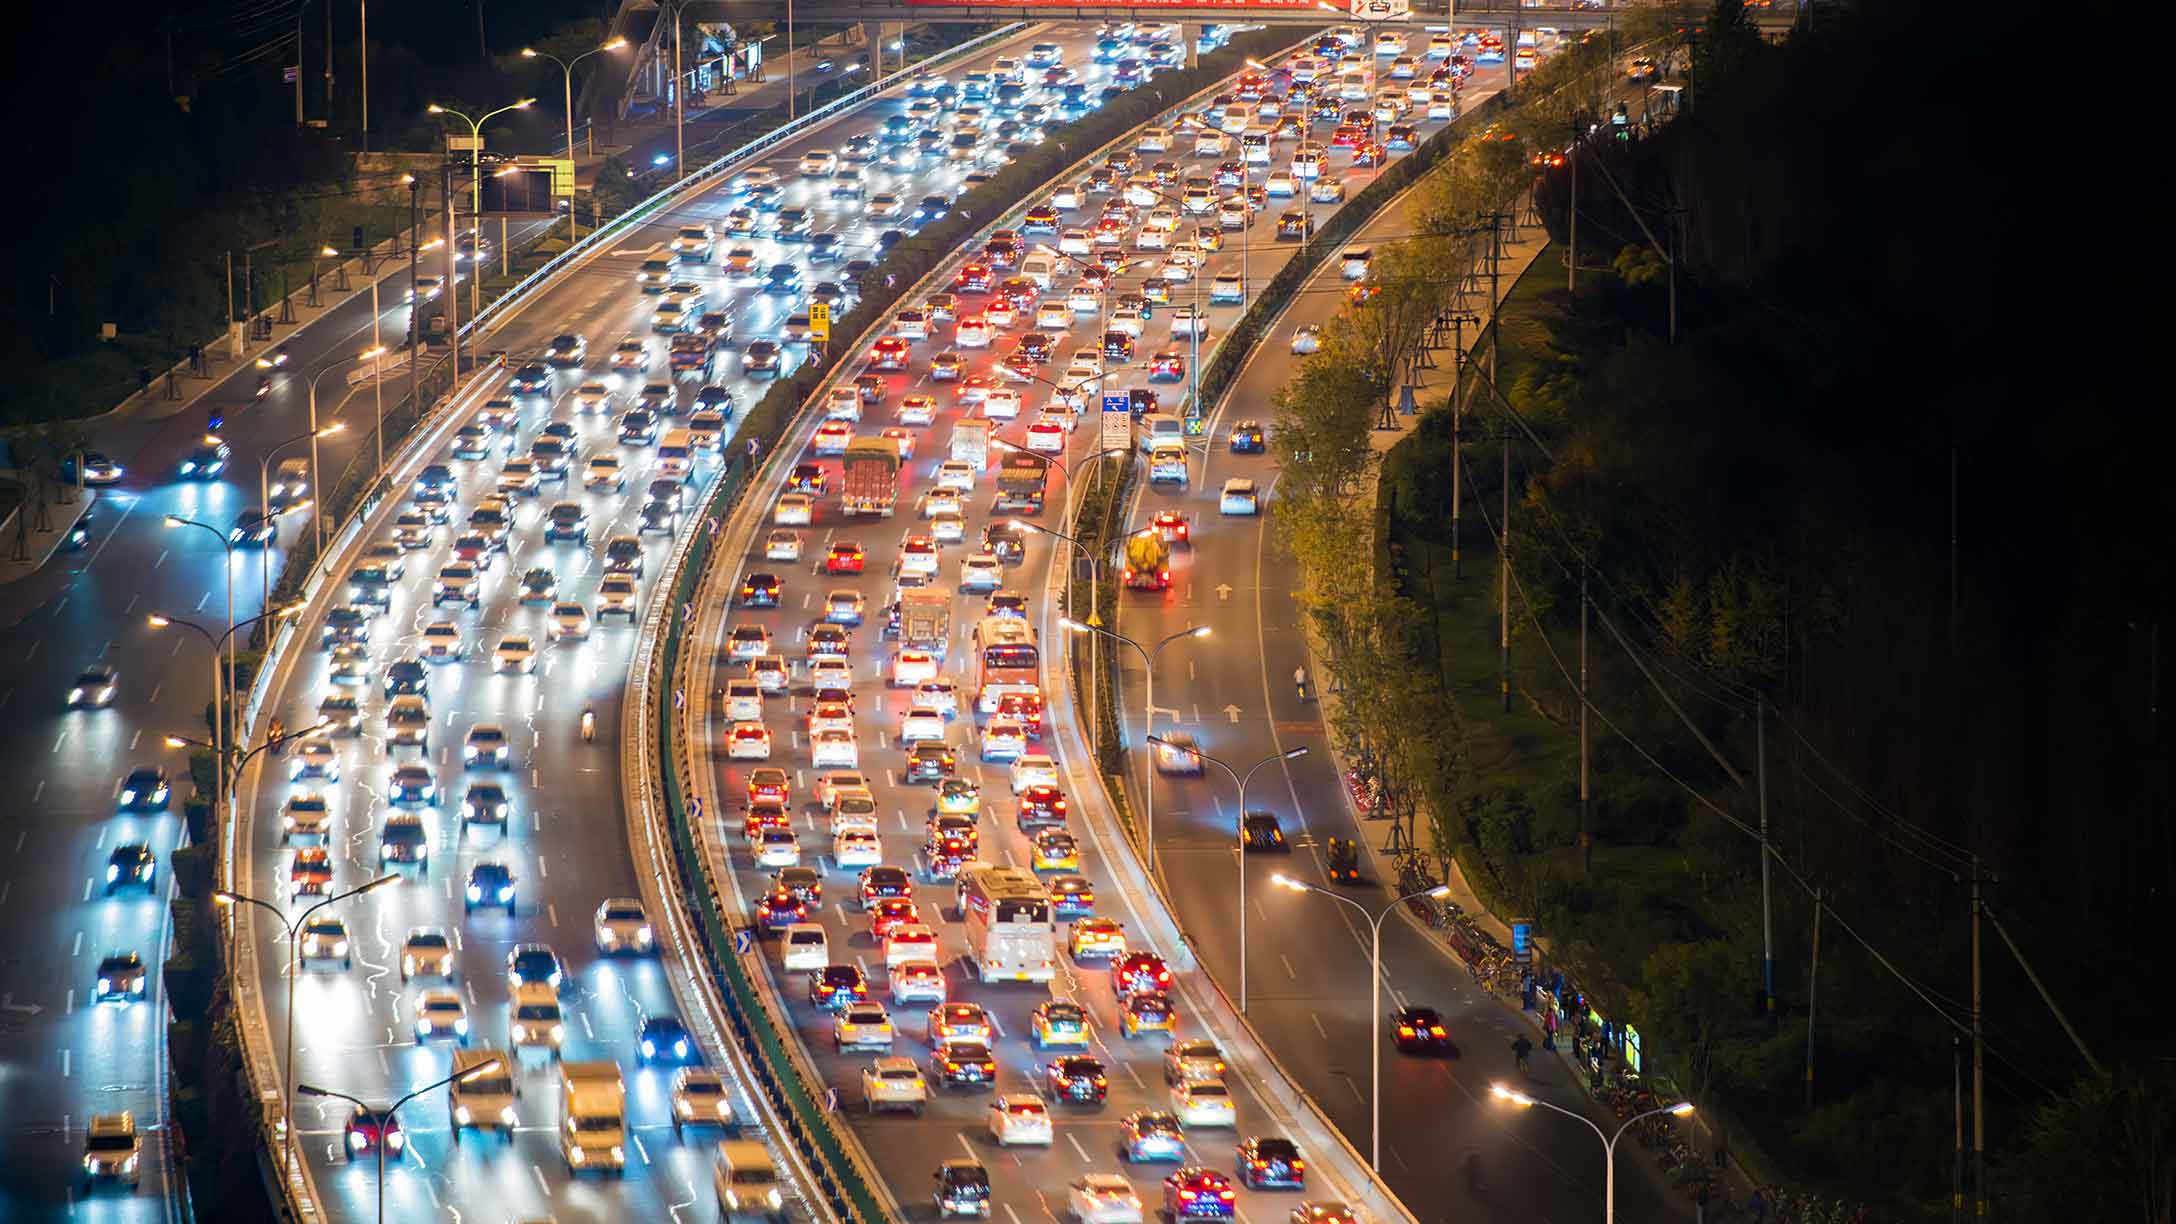}
        
        \textbf{Question:} \\
        Describe this photo in detail.
        \tcblower
        \textbf{Maya:} \\
        The image depicts a large, busy highway at night, with heavy traffic in both directions. There are numerous cars and trucks on the road, occupying almost all available lanes. The traffic appears to be moving slowly, with vehicles occupying the entire length of the highway. The scene is illuminated by the bright lights of the vehicles, as well as by the streetlights, creating a dynamic atmosphere. The highway extends into the distance, with no end in sight, highlighting the scale and congestion of this bustling transportation network.\\
        \textbf{LLaVA-7B:} \\
        The image depicts a busy highway filled with heavy traffic, including numerous cars and trucks. The highway is bustling with activity, as vehicles are seen in various positions, some moving and others waiting in line. The traffic is dense, with cars and trucks occupying almost every lane, creating a sense of congestion. The highway is surrounded by trees, adding a touch of nature to the urban landscape. The scene captures the essence of a typical day in a large city, with people commuting and traveling on the busy roads.\\
        \textbf{GPT4:} \\
        This is a top view photograph of a highway at night. The highway is divided into four sections. On the left side, there are three lanes of traffic approaching the camera and four lanes of traffic moving away from the camera. On the right side, there are four lanes of traffic approaching the camera and three lanes of traffic moving away from the camera. Most cars in the four-lane section moving away from the camera have their brake lights on, indicating a higher traffic density in the four-lane sections. Meanwhile, traffic appears to be lighter on the two three-lane sections. The four-lane highway is elevated compared to the three-lane highway, creating a visually distinct separation between the two sections. The lights alongside the highway are illuminated, providing a clear view of the road and cars. On the right side of the highway, there are trees, adding a touch of nature to the scene.
    \end{conversationbox}
    \caption{Comparison of model responses to visual questions on night highway traffic.}
    \label{fig:model_responses024_01}
\end{figure*}

\begin{figure*}[h]
    \centering
    \begin{conversationbox}{Asian Food}
        \includegraphics[width=0.7\linewidth]{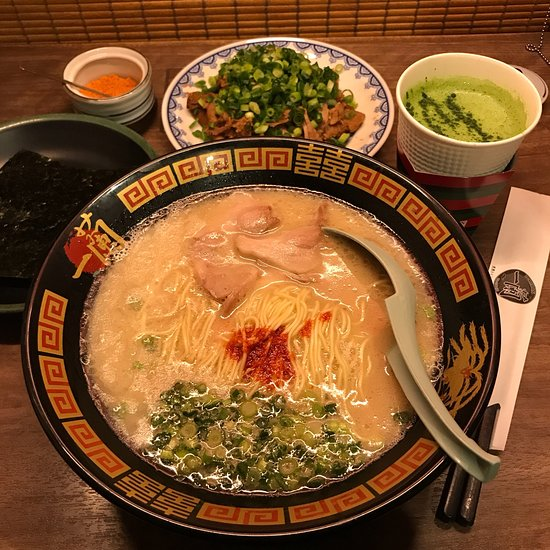}
        
        \textbf{Question:} \\
        Describe this photo in detail.
        \tcblower
        \textbf{Maya:} \\
        The image features a dining table with several bowls of food, including a large bowl of noodles and a few smaller bowls containing a variety of dishes, possibly Asian cuisine. The noodles are served in a bowl with vegetables, making it a delicious and healthy meal. There are also a couple of cups placed on the table, one near the top left corner and the other closer to the center. A spoon can be seen resting in one of the bowls, ready to be used. The table is set up with a variety of food options, making it an inviting scene for those who enjoy sharing and enjoying a meal together.\\
        \textbf{LLaVA-7B:} \\
        The image features a dining table with a variety of food items, including a large bowl of soup, a plate of noodles, and a bowl of vegetables. The soup is placed in the center of the table, while the noodles and vegetables are positioned around it. There are several bowls and cups scattered across the table, with some placed near the edges and others closer to the center. A spoon is also visible on the table, likely used for eating the soup. The table setting creates an inviting atmosphere for a meal.\\
        \textbf{GPT4:} \\
        This is a close-up photo of a meal at ICHIRAN. In the center, there is a chashu ramen bowl with a spoon. The ramen is seasoned with chili sauce and chopped scallions, and served with two pieces of chashu. To the right of the bowl, chopsticks are placed, still in their paper wrap, unopened. The ramen is accompanied by nori on the left side. On top, there are accompanying sides. From left to right, these include a bowl of orange spice (possibly garlic sauce), a plate of smoke-flavored stewed pork garnished with chopped scallions, and a cup of matcha green tea.
    \end{conversationbox}
    \caption{Comparison of model responses to visual questions on food details.}
    \label{fig:model_responses022}
\end{figure*}

% \begin{figure*}[t]
%   \centering
%   \fbox{\includegraphics[width=1\linewidth]{sec/assets/022.jpg}}
%   \caption{Example image from LLaVA-Bench (In-the-Wild) \citep{liu2023llava}.}
%   \label{fig:asianfood}
% \end{figure*}

\begin{figure*}[t]
  \centering
  \fbox{\includegraphics[width=1\linewidth]{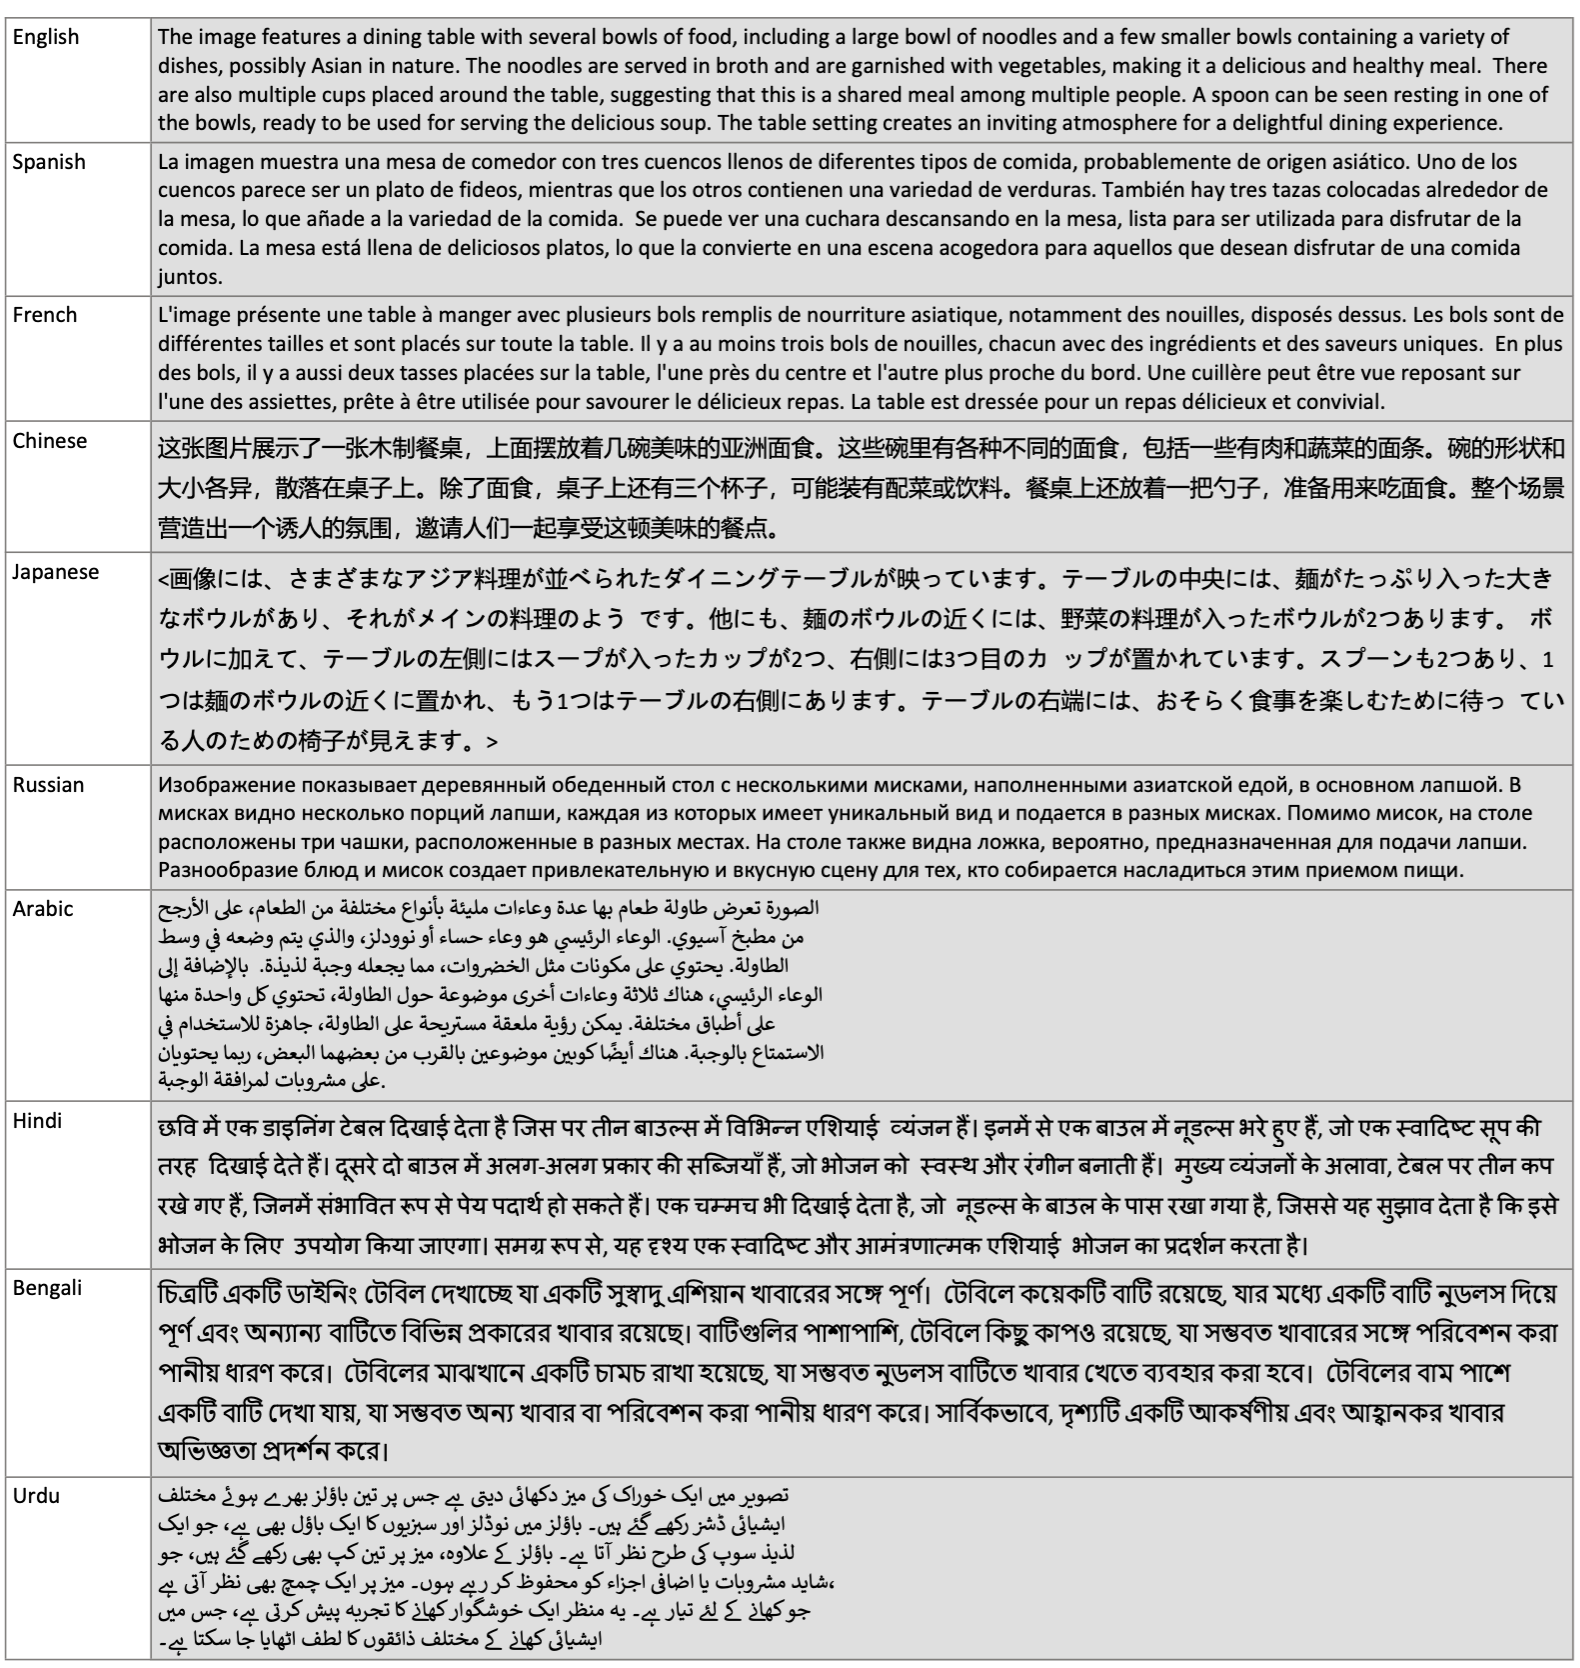}}
  \caption{Maya output for prompt (with image from Figure \ref{fig:asianfood}): Describe this photo in detail in \{language\}.}
  \label{fig:food_in_details}
\end{figure*}

% 
%Having the supplementary compiled together with the main paper means that:
% 
%\begin{itemize}
%\item The supplementary can back-reference sections of the main paper, for example, we can refer to \cref{sec:intro};
%\item The main paper can forward reference sub-sections within the supplementary explicitly (e.g. referring to a particular experiment); 
%\item When submitted to arXiv, the supplementary will already included at the end of the paper.
%\end{itemize}
% 
%To split the supplementary pages from the main paper, you can use \href{https://support.apple.com/en-ca/guide/preview/prvw11793/mac#:~:text=Delete%20a%20page%20from%20a,or%20choose%20Edit%20%3E%20Delete).}{Preview (on macOS)}, \href{https://www.adobe.com/acrobat/how-to/delete-pages-from-pdf.html#:~:text=Choose%20%E2%80%9CTools%E2%80%9D%20%3E%20%E2%80%9COrganize,or%20pages%20from%20the%20file.}{Adobe Acrobat} (on all OSs), as well as \href{https://superuser.com/questions/517986/is-it-possible-to-delete-some-pages-of-a-pdf-document}{command line tools}.
